# Supplementary material for: Waterberry Farms: A Novel Benchmark For Informative Path Planning
Source: arXiv:2305.06243 source file (2023-05-10)
Supplement: Supplementary file 1 [file AdditionalRelatedWork.tex]

---------------- here ---------

Dutta et al.~\cite {dutta2020multi} presented a continuous informative multi-robot region partitioning algorithm in a foreign environment. In the proposed algorithm, the Voronoi regions will be re-calculated (so is the path planning) every time the robots are in communication range with one another, in which they relay each one's perception of the world, points of interest, and whether the budget limit has reached. In addition, each robot is equipped with a laser rangefinder with a given detection range to detect obstacles that the robot may encounter in the environment. The model that the proposed algorithm solves is the case when robots get dropped off onto an unknown terrain for exploration. 
Extending their previous work, Dutta et al. studied multi-robot sampling using the Decentralized Markov Decision Process (MDP) \cite{dutta2021opportunistic} under a similar environment as in their previous work \cite{dutta2020multi}. That is, a) each robot is given a region for the sampling task, b) robots are assumed to have intermittent communication with each other, but when they do, they share past observations and use a Gaussian mixture to update their perception of the world. MDP uses Gaussian Process generated from training data to calculate the initial rewards. 

In~\cite{binney2010informative}, Binney et al. proposed an algorithm for Autonomous Underwater Vehicle (AUV) path planning. The AUV is assumed to only communicate the observations when it re-surfaces, and share the readings to improve the path dynamically. Therefore, one of the main contributions that Binney et al. made was to use the time-window concept to avoid high traffic areas at certain times to prevent any collision that might happen with the boats when the AUV re-surface. Additionally, Binney et al. modified the recursive greedy algorithm for path planning to fit the AUV case, another study on informative and adaptive path planning. 

Cui et al.~\cite{cui2015mutual} also studied the Autonomous Underwater Vehicle (AUV) and developed a multi-robot adaptive informative path planning algorithm. They used the Selective Basis Function Kalman filter in a distributed manner to estimate the scalar field model on the collected samples, utilizing the consensus algorithm. Additionally, they used the multi-dimensional RRT* algorithm to calculate the next sampling point for the AUVs. 
One of the limitations of the AUVs is the limited time these vehicles spend underwater. The longer the AUV stays underwater, the larger the number of samples; with larger sample set, the algorithms take more time to find a solution. The most commonly used regression technique for spatial modeling is Gaussian Process (GP). Therefore, Chen et al. \cite{chen2019long} proposed a solution to the issue mentioned above by using a sparse variant of Gaussian Process (GP) called Streaming Sparse GP (SSGP). The proposed SSGP can handle streaming data in an online and incremental manner, which allows the AUVs to stay longer underwater. 
On the other hand, Wei et al. \cite{wei2020informative} suggested using Reinforcement Learning (RL) for Informative Path Planning. According to Wei et al., an RL-based solution doesn't require re-executing the algorithm like other algorithms when the input parameters change. This characteristic of the RL-based solution makes the proposed solution stand out from other solutions. 
Just as \cite{wei2020informative} presented a solution that uses RL, Said et al. also suggested an RL solution that uses a concept of Mean Field Games (MFG) to scale out the algorithm to a larger number of robots \cite{said2021multi}. In addition to using MFG to learn a function of the mean action of all robots, Said et al. used a Recurrent Neural Network (RNN) with MFG for better information sampling.
Additionally, Yang et al. \cite{yang2018mean} has also studied RL in a similar context and proposed using the Mean Field theory to solve the scalability problem of having many agents in a Multi-Agent Reinforcement Learning (MARL) environment. Yang et al. offered a way to average out the effect of agents on one another, hence developing mean-field Q-Learning and mean-field Actor-Critic algorithms. 
Sometimes, it's essential to consider the space and time of the environment for path planning. For example, if we want to monitor oil spill distribution in the ocean, it's not sufficient to only know where the spill occurred, as the oil will spread out to larger areas with time. Therefore,
Chen et al. \cite{chen2019multi} took a different direction in their approach to informative path planning by using the Monte Carlo Tree Search algorithm (MCTS). Using MCTS helps in the exploration and exploitation of the environment and allows to update the current model dynamically, therefore considering the space and time in their calculations.
On the other hand, Coverage Path Planning (CPP) has been extensively studied in the past years under the assumption that the robot has unlimited power. Sharma et al. \cite{sharma2019optimal} researched CPP for robots with energy constraints. Their proposed algorithm aims to minimize the total distance the robot travels and the number of times it returns to the charging station. Their algorithm achieves both mentioned objectives in O(log(B/L) (where B is the budget unit distance and L is the length of the cell in the environment) and uses Depth First Search (DFS) to traverse the environment. 
Wheeled Mobile Robots (WMRs) navigation in agriculture has many challenges. The terrain, for example, is a complex structure that may include many obstacles and crops that the robot needs to be careful not to damage. Robots need to have a good perception of the environment and to be able to conclude the next traveling point. The accuracy of the algorithms is an essential factor in this problem, as allowing errors may lead the robots to get stuck or lost in the field. Gao et al. \cite {gao2018review} have reviewed the standard algorithms in mapping, localization, path planning, and obstacle avoidance and wrote about the advantages and disadvantages of each of them. 
Another study on robots in the agricultural environment has been researched by Rold{\'a}n et al. \cite {roldan2018robots} who summarized the applications of robots in the fields and greenhouses. They looked into the Unmanned Ground Vehicle (UGV) and Unmanned Aerial Vehicle (UAV) for single robot applications and when having a fleet of robots set up that have a mix of UAVs and UGVs in a multi-robot environment and the communications that these robots could make.

Now that we have shown lots of work in the literature on path planning algorithms for single and multi-robot environments, we shift gears just a bit to discuss methods and applications we can use to benchmark algorithms. After all, what good is the algorithm if we can't test its performance and efficiency? 
Toma et al. \cite {pathBench_Toma} presented an application called PathBench. PathBench is an open-source application for developing, visualizing, training, testing, and benchmarking existing and future path planning algorithms. According to \cite{pathBench_Toma}, PathBench supports A*, wavefront, rapidly-exploring random trees, value iteration networks, and gated path planning networks. PathBench uses several criteria in benchmarking, such as path length, success rate, computational time, and path deviation. Although PathBench seems an exciting application that covers many things, it isn't the only application for benchmarking. Heiden et al. \cite {heiden2021bench} presented another open-source application called Bench-MR, designed for sampling-based motion planning for nonholonomic, wheeled mobile robots. According to Heiden et al. Bench-MR is easy to use and provides many algorithms, extend functions, collision checkers, etc., that help researchers design and test their algorithms.
